# Supplementary material for: Bi-tuning of Pre-trained Representations
Source: arXiv:2011.06182 source file (2020-11-12)
Supplement: Supplementary file 1 [file supp.tex]

\iffalse

\bibliography{../ref/JZhong.bib}

\fi

\section{Key Generating Mechanism and Implements}

\subsection{Momentum Contrast}

Momentum Contrast (MoCo)~\cite{he2019momentum} is a general mechanism for using contrastive loss. The main idea in MoCo is that producing encoded keys on-the-fly via a momentum-updated encoder and maintaining a queue to support sampling operations. Thus, the memory consumption in MoCo does not depend on the size of the training set (while a memory bank~\cite{wu2018unsupervised} will store the whole dataset). In Section 4, CORE chooses MoCo as our default setting in the experiments.

Formally, denoting the momentum-updated encoder as $f_k$ with parameters $\theta_k$. Likewise, denoting the backbone encoder as $f_q$ with parameters $\theta_q$. $\theta_k$ is updated by:

\begin{equation}\label{moco}
	\theta_k \leftarrow m\theta_k + (1-m)\theta_q
\end{equation}

Here we set the momentum coefficient $m=0.999$. To fit the CORE framework, we reorganize the queues in MoCo for items in each category separately. Moreover, two contrastive mechanisms in CORE are performed on different levels, and we maintain two groups of queues respectively.

\subsection{Memory Bank}

CORE is a general framework, which is not bundled to any special key generating mechanism (MoCo). The memory bank proposed by \cite{wu2018unsupervised} generating encoded keys via momentum-updated snapshots of all items in the training set. Keys for each mini-batch are uniformly sampled from the memory bank. Compared to MoCo, maintaining a memory bank is more computation-efficient with more memory required. Similar to Eq. \eqref{moco}, snapshots here updated by:

\begin{equation}\label{mb_z}
	\mathbf{z}_i^k \leftarrow m\mathbf z_i^k + (1-m)\mathbf z^q_i
\end{equation}

\begin{equation}\label{mb_h}
	\mathbf{h}_i^k \leftarrow m\mathbf h_i^k + (1-m)\mathbf h^q_i
\end{equation}

Notations follow Section 3. Here we set the momentum coefficient $m=0.5$ \cite{wu2018unsupervised}.  Other hyper-parameters are the same as Section 4. We evaluate CORE with a memory bank on CUB~\cite{cub200-WelinderEtal2010} with the same configurations in Section 4. The results shown in table \ref{table:mecha} suggest that the key generating mechanism in CORE can be implemented by some variants with similar performance.

\begin{table*}[!tbp]
	\addtolength{\tabcolsep}{2pt}
	\centering
	\begin{tabular}{ccccccc}
	  \toprule
	  \multirow{2}*{Key generating mechnism} & \multicolumn{4}{c}{Sample Rate} \\
	    & $25\%$ & $50\%$ & $75\%$ & $100\%$\\
	  \midrule
	  MoCo        & $49.25\pm$0.23 & $66.88\pm$0.13 & $74.27\pm$0.05 & $77.12\pm$0.23  \\
	  Memory bank & $50.01\pm$0.55 & $66.69\pm$0.26 & $74.22\pm$0.31 & $77.62\pm$0.29  \\
	  \bottomrule
	  
 	\end{tabular}
 
	\caption{Top-1 accuracies (\%) of CORE with memory bank on CUB using ResNet-50 pretrained via MoCo as the backbone. Performance is close in both methods. Key generating mechanisms in CORE only have limited effects on the final performance in the supervised paradigm. MoCo is recommended regarding its extensibility. }
	\label{table:mecha}
\end{table*}

\section{Full Results of Ablations in Section 4}

Due to space limitation in the main text, standard deviations in Table 3 (ablations of number $K$) and Table 5 (ablations of the projectors) are omitted. The following Table \ref{table:fksm} is the full extension to Table 3 in Section 4, Table \ref{table:fdim} is the full extension to Table 5 in Section 4.

\begin{table*}[!htbp]
	\centering
	\addtolength{\tabcolsep}{2pt}
	\centering
	
	%\vspace{-3pt}
	\begin{tabular}{ccc}
	\toprule
	\multirow{2}*{Key sampled per class} & \multicolumn{2}{c}{Sampling Rates} \\
	 & 25\% & 100 \% \\
	\midrule
	1        & $48.93\pm$0.37  &  $75.90\pm$0.35 \\
	2        & $49.25\pm$0.23  &  $76.45\pm$0.22 \\ 
	4        & $49.09\pm$0.19  &  $76.26\pm$0.45 \\
	8        & $47.94\pm$0.12  &  $76.41\pm$0.09 \\
	16       & $47.65\pm$0.71  &  $76.40\pm$0.34 \\
	32       & $47.78\pm$0.31  &  $77.12\pm$0.23 \\
	64       & $44.10\pm$0.60  &  $76.23\pm$0.45 \\   
	 \bottomrule
 	\end{tabular}
 	%}
	\caption{Comparison of different numbers of sampled keys, on 25\% and 100\% ratio of CUB (200 categories), indicates that there exists a trade-off between sampling stochasticity and a large number keys. (backbone ResNet50 via MoCo). Note that keys may be duplicate when the number of sampled keys is larger than dataset size.}
	\label{table:fksm}
	% \vspace{-10pt}
\end{table*}

\begin{table*}[!htbp]
	\centering
	\addtolength{\tabcolsep}{2pt}
	\centering
	
	%\vspace{-3pt}
	\begin{tabular}{ccc}
	\toprule
	\multirow{2}*{dim} & \multicolumn{2}{c}{projector} \\

	 & from scratch  & retraining  \\
	\midrule
	32        & $90.55\pm$0.16  &  - \\
	64        & $90.65\pm$0.15  &  - \\ 
	128       & $90.78\pm$0.19  &  $90.88\pm$0.13 \\
	256       & $90.79\pm$0.23  &  - \\
	512       & $90.81\pm$0.06  &  - \\
	1024      & $91.01\pm$0.26  &  - \\
	 \bottomrule
 	\end{tabular}
 	%}
	\caption{Top-1 accuracies (\%) on Cars with different projection head $g(\cdot)$ (backbone ResNet50 pretrained via MoCo) . Here ‘-’ denotes that these results are not available since the dimension of MoCo is $128$. }
	\label{table:fdim}
	% \vspace{-10pt}
\end{table*}
